# Supplementary material for: Towards Content-based Pixel Retrieval in Revisited Oxford and Paris
Source: arXiv:2309.05438 source file (2023-09-11)
Supplement: Supplementary file 1 [file label_instruction.pdf]

# 1 Recognize

- You should **identify the query** object in the labeling image firstly. You can zoom in and zoom out the query and the labeling image for observation. If you can not find the query object in the labeling image in 3 minutes, report and skip this image.

Before labeling, you should identify the target object firstly.

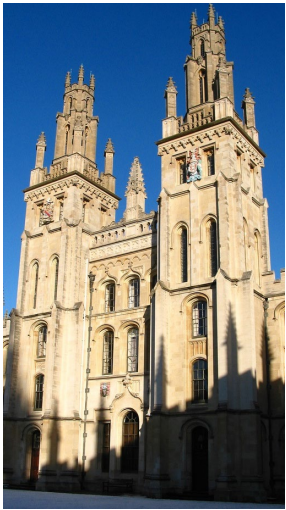

Query

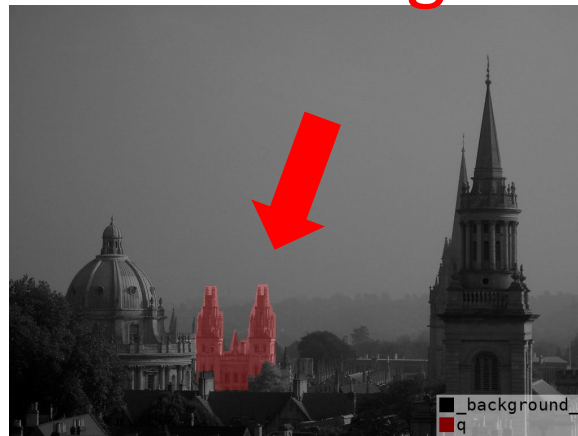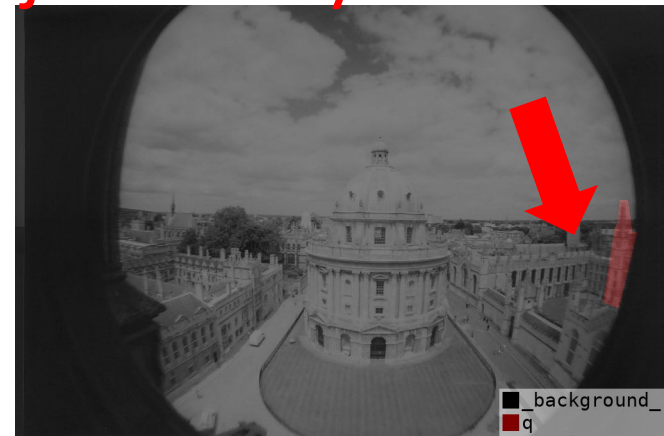

Labeling images

## 2 Label all the pixels

- You should label all the pixels belonging to the identified object. Due to the *viewpoint* and *time* change, the same object in two images may be **slightly different** (no pixel to pixel correspondence). Label it as long as you judge that a pixel is depicting the target object.

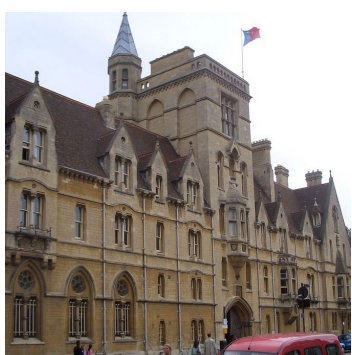

Query

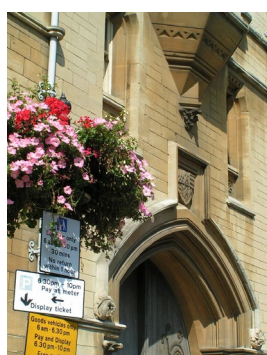

Positive image

OK

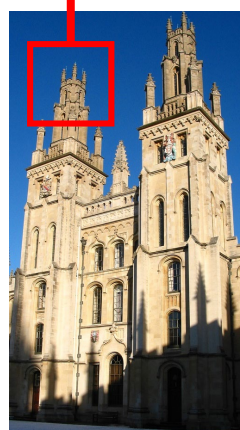

Query

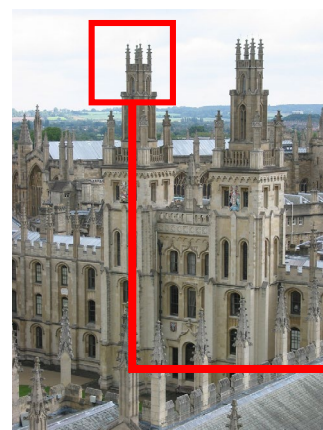

Positive image

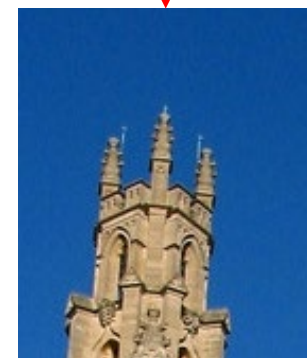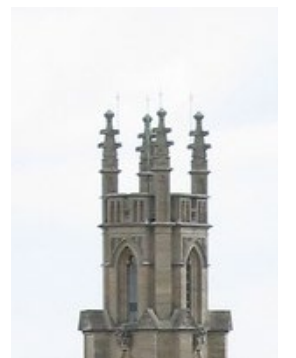

OK



# 3 Understand the query

- The target object may connect to or is a part of another object. Although we have crop the background, there may still be unrelated pixels. Judge the intention of the query example by yourselves.

Query object is a part of another object

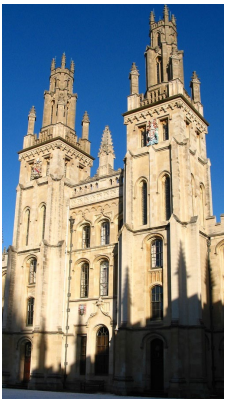

Query

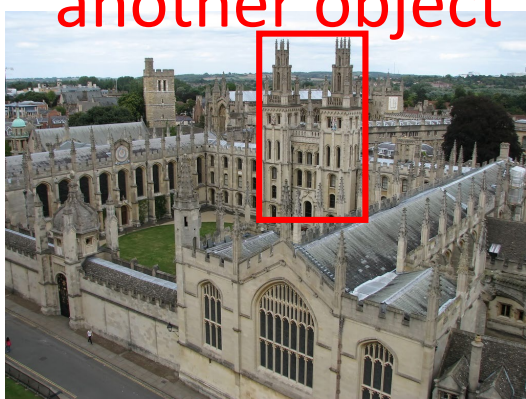

Labeling image

Query object is a part of another object

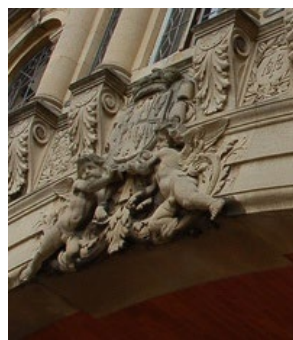

Query

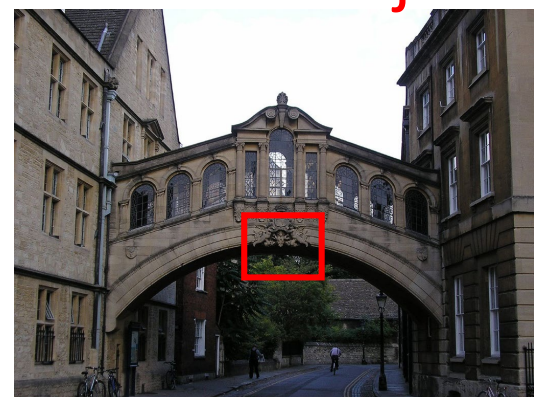

Labeling image

# 4 occlusion

- A part of the target object may be occluded by objects like a fence and window. You do not need to remove all the occlusion pixels. However, there should be only one clear salient object in the mask region. Remove all the pixels that violate this rule.

Allow this kind of occlusion

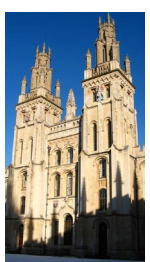

Query

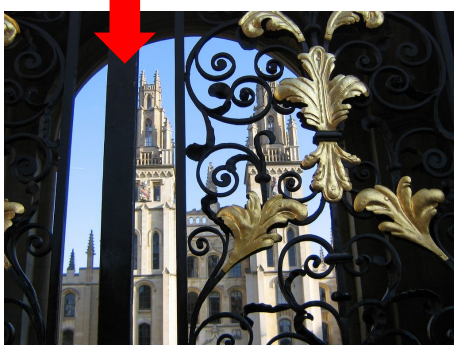

Labeling image

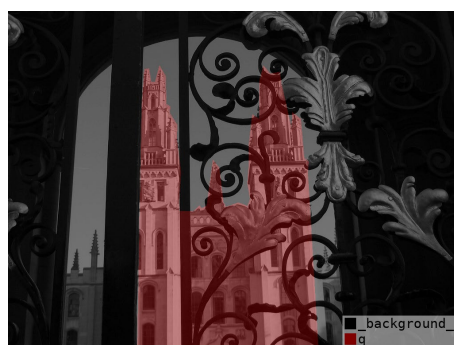

Labeled example

Remove this kind of occlusion

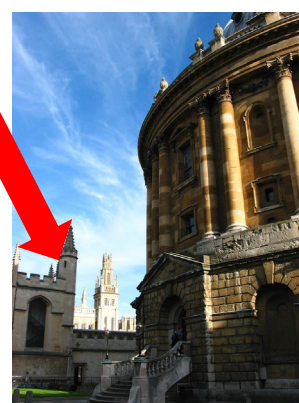

Labeling image

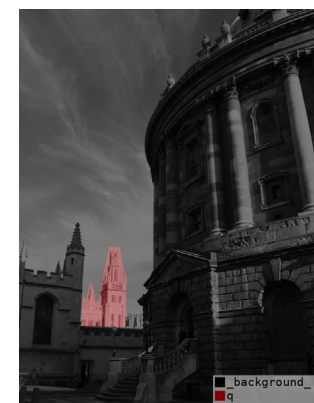

Labeled example
